# Supplementary material for: Level-S$^2$fM: Structure from Motion on Neural Level Set of Implicit Surfaces
Source: arXiv:2211.12018 source file (2023-03-27)

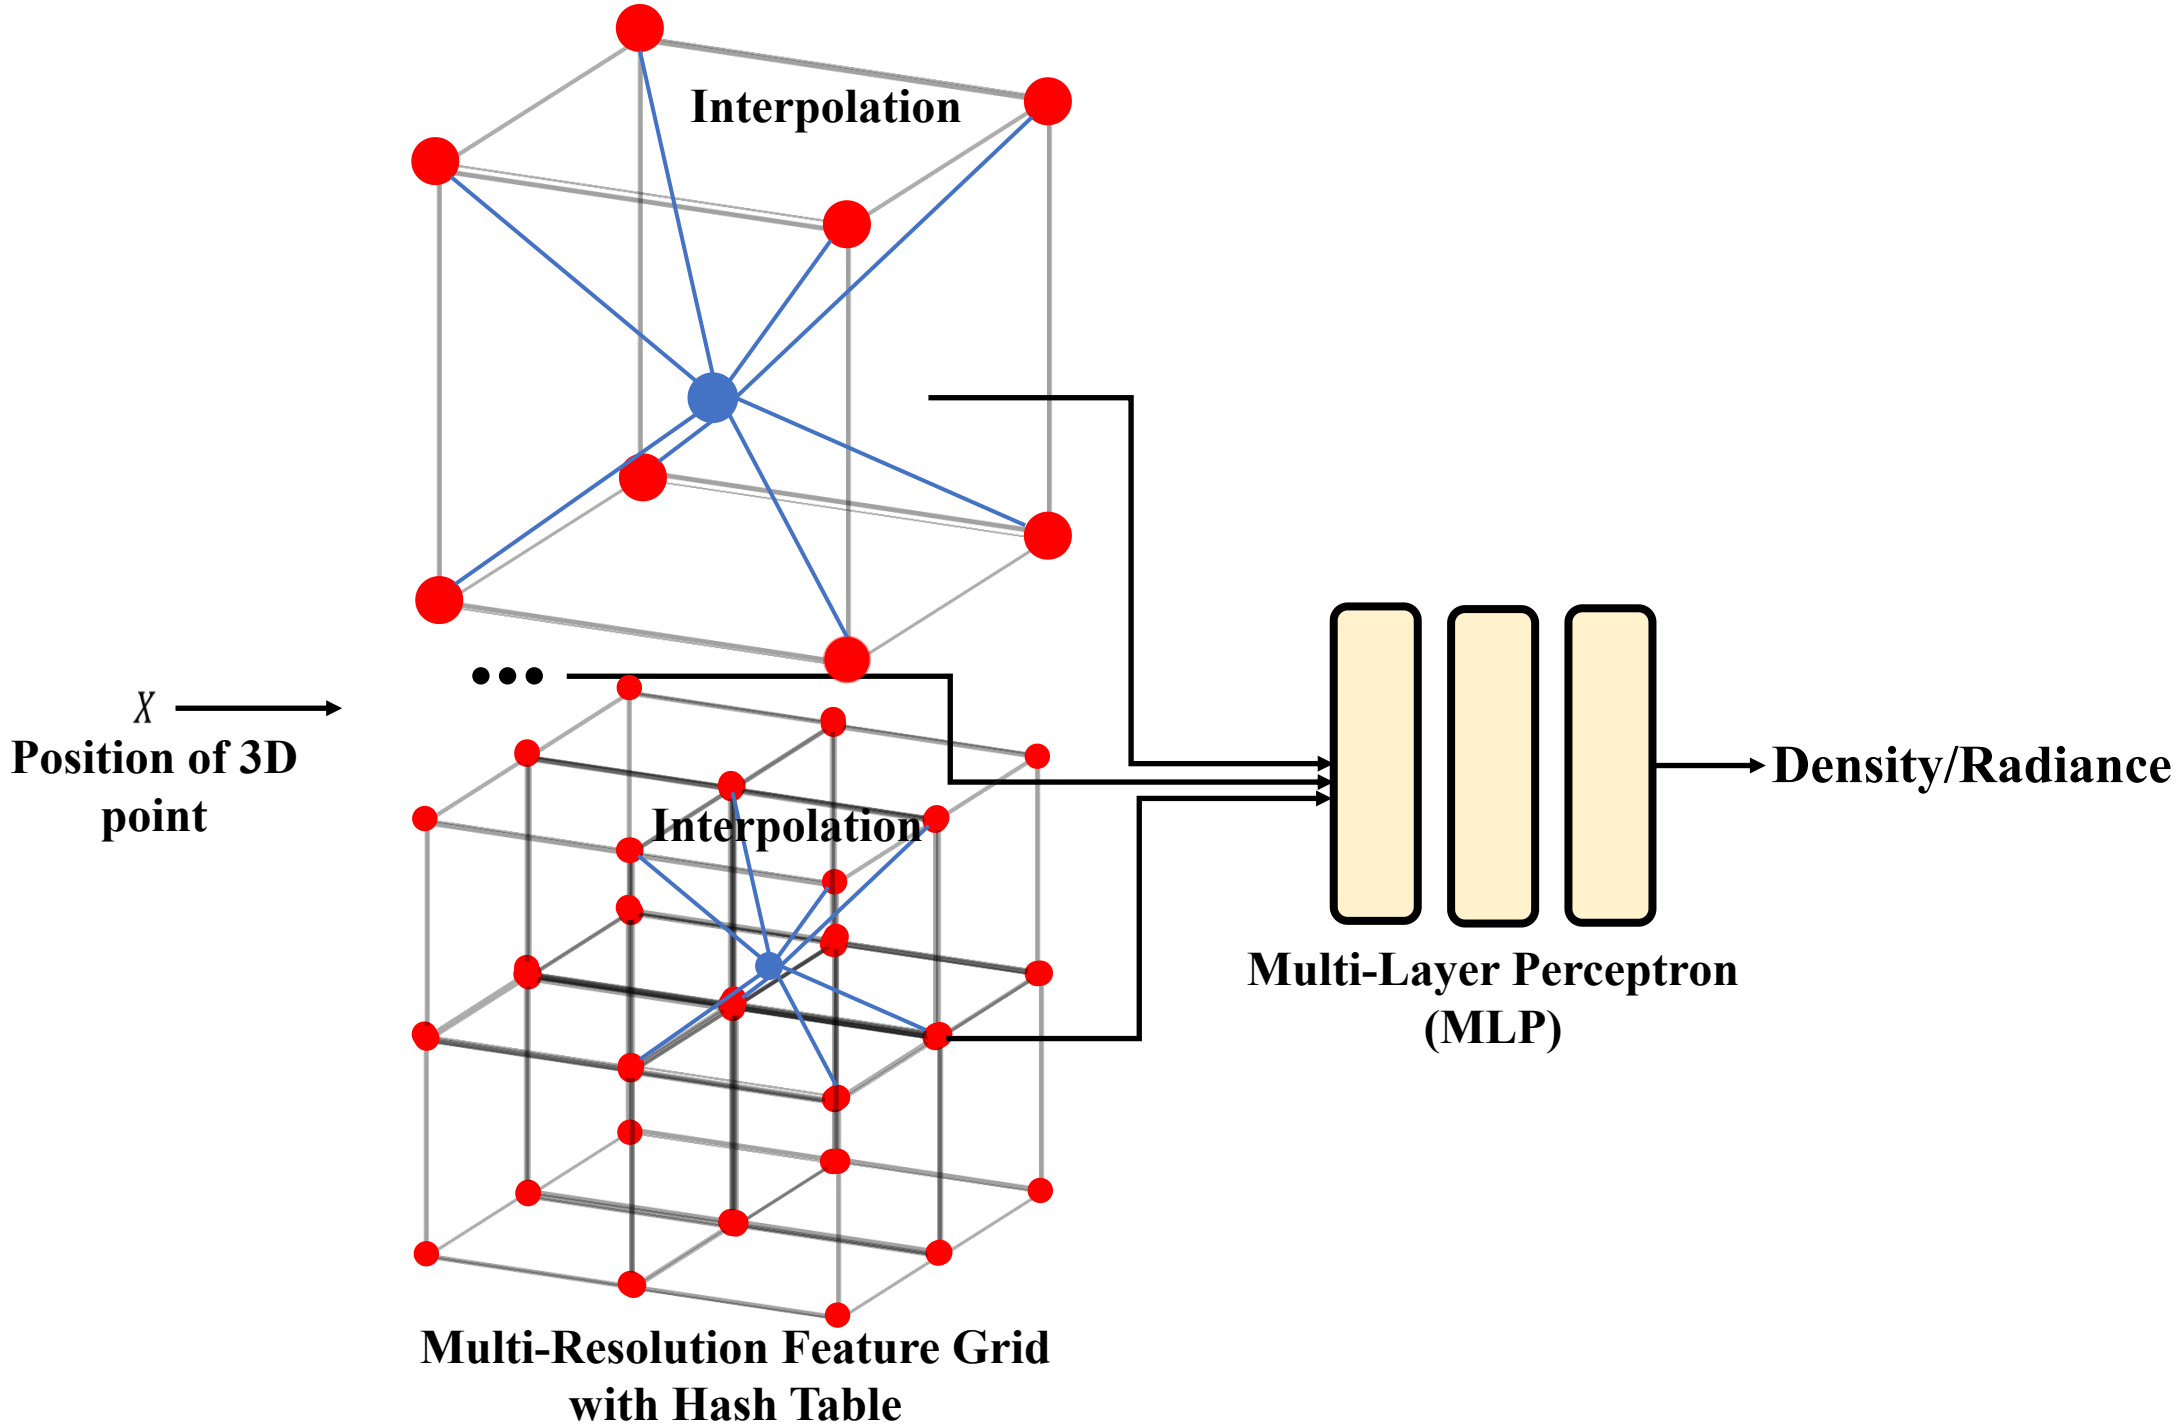

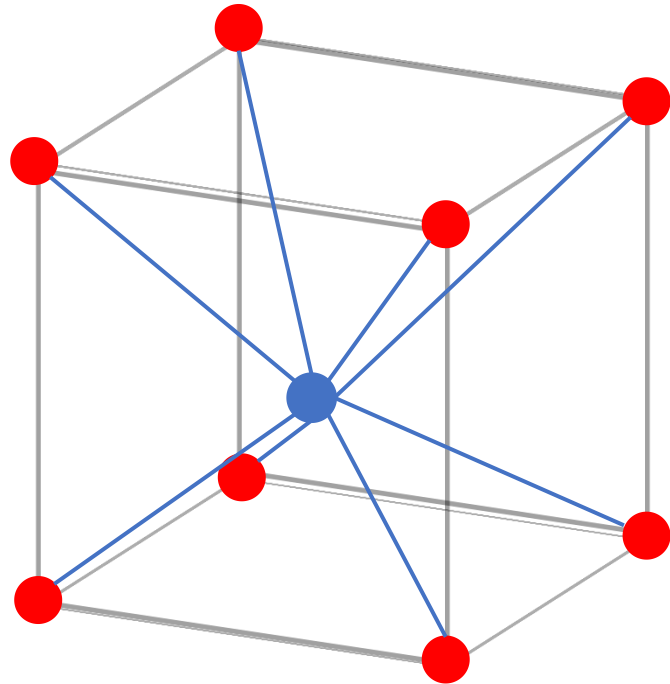

...

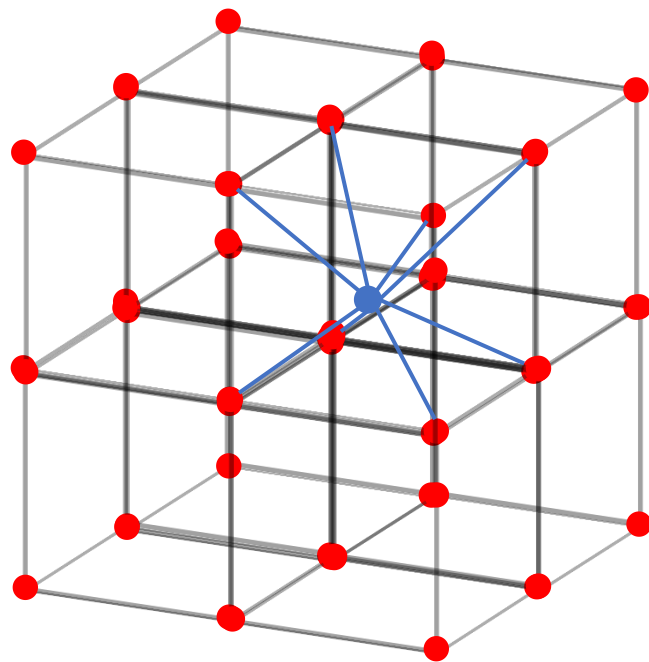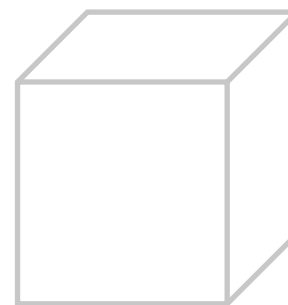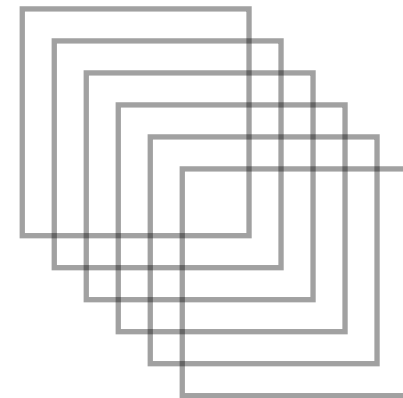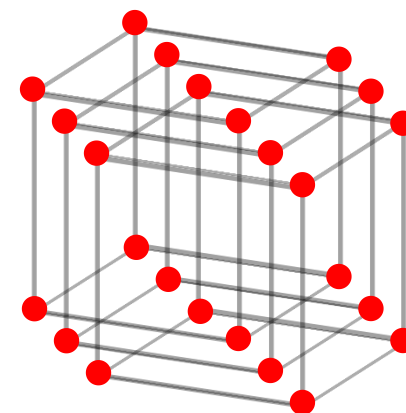

Supplement: Supplementary file 1 [file Supplementary_cut.pdf]
